# Supplementary material for: Planetesimal formation via the streaming instability with multiple grain sizes
Source: arXiv:2305.11297 source file (2023-09-27)
Supplement: Supplementary file 1 [file 5_appendix.tex]

\section{Appendix, if needed}
